# Supplementary material for: Diverse Distributions of Self-Supervised Tasks for Meta-Learning in NLP
Source: arXiv:2111.01322 source file (2021-11-02)
Supplement: Supplementary file 1 [file datasets.tex]

\begin{table*}[tb!]
\centering
\resizebox{\linewidth}{!}{%
% \scalebox{0.57}{
\begin{tabular}{ccccccc}
\Xhline{2\arrayrulewidth}
% \multicolumn{16}{c}{\textbf{Natural Language Inference}}                                              \\ \Xhline{2\arrayrulewidth}
% \multicolumn{1}{l}{} & \multicolumn{5}{c}{\textbf{MNLI}}              & \multicolumn{5}{c}{\textbf{QNLI}}               & \multicolumn{5}{c}{\textbf{RTE}}               \\ 
Dataset & Labels & Training Size & Validation Size & Testing Size  & Source\\ \hline

Amazon Review Domains & 2 & 800 & 200 & 1000 & \cite{blitzer2007biographies} \\ \hline
% CoLA & 2 & 8551 & 1042 & --- & \cite{warstadt2019neural} \\ \hline
MRPC & 2 & 3669 & 409 & --- & \cite{dolan2005automatically} \\ \hline
% QNLI & 2 & 104744 & 5464 & ---  & \cite{rajpurkar2016squad,wang2018glue} \\ \hline
% QQP & 2 & 363847 & 40431 & ---  & \cite{wang2018glue} \\ \hline
RTE & 2 & 2491 & 278 & ---  & \cite{dagan2005pascal,haim2006second,giampiccolo2007third,giampiccolo2008fourth} \\ \hline
% SNLI & 3 & 549368 & 9843 & ---  & \cite{bowman2015snli} \\ \hline
% SST-2 & 2 & 67350 & 873 & ---  & \cite{socher2013recursive} \\ \hline
% MNLI \tiny{(m/mm)} & 3 & 392703 & 19649 & ---  & \cite{williams2017broad} \\ \hline
Scitail & 2 & 23,596 & 1,304 & 2,126  & \cite{khot2018scitail} \\ \hline
Airline & 3 & 7320 & --- & 7320  & \url{https://www.figure-eight.com/data-for-everyone/} \\ \hline
Disaster & 2 & 4887 & --- & 4887  &  \url{https://www.figure-eight.com/data-for-everyone/} \\ \hline
Political Bias & 2 & 2500 & --- & 2500  & \url{https://www.figure-eight.com/data-for-everyone/} \\ \hline
Political Audience & 2 & 2500 & --- & 2500  & \url{https://www.figure-eight.com/data-for-everyone/}\\ \hline
Political Message & 9 & 2500 & --- & 2500  & \url{https://www.figure-eight.com/data-for-everyone/} \\ \hline
Emotion & 13 & 20000 & --- & 20000  & \url{https://www.figure-eight.com/data-for-everyone/} \\ \hline
CoNLL & 4 & 23499 & 5942 & 5648  & \cite{sang2003conll} \\ \hline
MIT-Restaurant & 8 & 12474 & --- & 2591  & \cite{liu2013asgard} \url{https://groups.csail.mit.edu/sls/downloads/restaurant/} \\ \hline
% \Xhline{2\arrayrulewidth}
\end{tabular}
}
\caption{Dataset statistics for all the datasets used in our analysis. "-" represent data that is either not available or not used in this study.}
\label{tab:dataset}
\end{table*}
