# Supplementary material for: Diverse Distributions of Self-Supervised Tasks for Meta-Learning in NLP
Source: arXiv:2111.01322 source file (2021-11-02)
Supplement: Supplementary file 2 [file intra_clus.tex]

\begin{table*}[t]
\centering

 % we want center vertical alignment

\begin{tabularx}{\textwidth}{|c|>{\raggedright}X|}
\hline
\textbf{} & \textbf{ Example Tasks:} \tabularnewline
\hline
Intra Cluster Task Sample 1  & \textbf{\emph{rents}}
\begin{itemize}
    \item Apartment [unused1] in Vegas grew by 5.8 percent over the 12 months that ended in the third quarter 2017, according to Axiometrics. 
    \item Most of the cottages are still occupied – they are now owned by the National Trust, which [unused1] them out. 
    \end{itemize}
    \textbf{\emph{million}}
\begin{itemize}
    \item Considering you have a [unused1] home security possibilities, how can you choose the most beneficial security business for your needs? 
    \item Four [unused1] beneficiaries do not have bank accounts. 
    \end{itemize}
        \textbf{\emph{bankrupts}} 
\begin{itemize}
    \item With discharged [unused1], however, many extra features such as a pre-purchase approval may not be available. 
    \item When choosing a lender, consider looking for one that not only offers loans to discharged [unused1], but also one that has a good track record and reputation.
    \end{itemize}
   \tabularnewline
   
   \hline
Intra Cluster Task Sample 2  & \textbf{\emph{despaired}} 
\begin{itemize}
    \item My old friends [unused1] - I received letters pleading with me not to carry on. 
    \item They are just waiting for you to knock on their door so don't get [unused1]. 
    \end{itemize}
    \textbf{\emph{depleted}} 
\begin{itemize}
    \item If your life has been overcome with gambling debts, the associates at Kevin Thatcher can help you get back on your feet, so you can focus on your health instead of your [unused1] wealth. 
    \item When I spend any length of time somewhere flat, grey, or lacking in trees, I feel [unused1]. 
    \end{itemize}
        \textbf{\emph{overlaid}} 
\begin{itemize}
    \item Each person’s clothing is [unused1] with images of the critical assets and essential services UGL provides to sustain and enhance the environment in which we live. 
    \item So maybe, just maybe, it isn’t so bad that no efficient film director fast-forwarded those endless page-flipping scenes, or [unused1] them with victorious soundtracks. 
    \end{itemize}
   \tabularnewline

\hline
\end{tabularx}
\caption{Word Sampling tasks created with words from  same cluster }
\label{tab:tasks}
\end{table*}
