# Supplementary material for: Diverse Distributions of Self-Supervised Tasks for Meta-Learning in NLP
Source: arXiv:2111.01322 source file (2021-11-02)
Supplement: Supplementary file 3 [file words.tex]

\begin{table}[t]
\begin{center}
\resizebox{\linewidth}{!}{%
 \begin{tabular}{|c | c |} 
 \hline
 \textbf{Clusters}  & \textbf{Words} \\
 \hline
 1 & Blogging, chromebook, blogposts,Freelancer, HyperText \\ 
 \hline
 2 & symptons, itchiness, septic, vaccinate, hospital \\
 \hline
 3 & Lahore , Madras, Rajasthan, Dhaka, Bhubaneshwar \\
 \hline
 4 & infinity, curve, fibonacci, Bayes, neutrino  \\
 \hline
 5 & you, would, shall, dont, when\\
 \hline
\end{tabular}
}
\caption{Top words among each cluster}
\label{tab:words}
\end{center}
\end{table}
